# Supplementary material for: On the instability of embeddings for recommender systems: the case of Matrix Factorization
Source: arXiv:2104.05796 source file (2021-04-12)
Supplement: Supplementary file 1 [file appendix.tex]

\section{Algorithms popularity bias}
\label{appendix:algo-popularity-bias}

We evaluate the popularity bias of the algorithms, considering the percentage of popular and unpopular item recommendations, \textit{i.e.} of recommendations of items belonging to the long tail and short head.
\begin{figure*}[h]
    \centering
    \begin{subfigure}[b]{0.32\textwidth}
        \caption{Epinions}
        \includegraphics[width=0.95\textwidth, keepaspectratio]{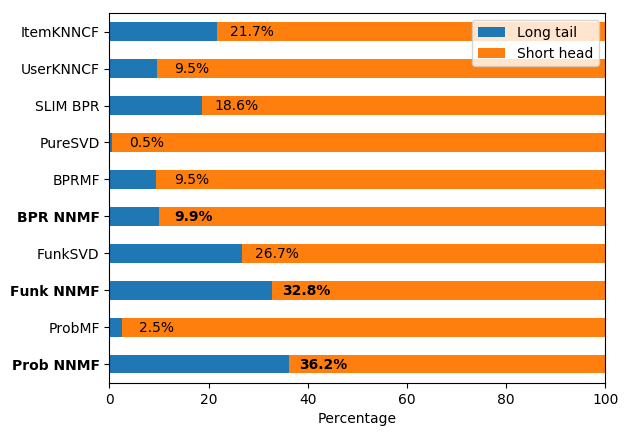}
    \end{subfigure}
    \begin{subfigure}[b]{0.32\textwidth}
        \caption{Pinterest}
        \includegraphics[width=0.95\textwidth, keepaspectratio]{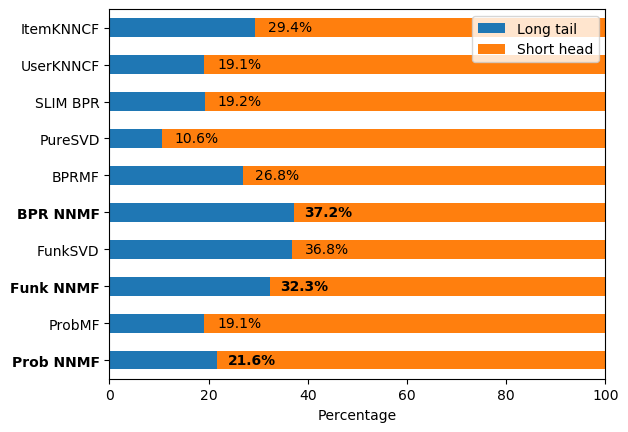}
    \end{subfigure}
    \centering
    \begin{subfigure}[b]{0.32\textwidth}
        \caption{BookCrossing}
        \includegraphics[width=0.95\textwidth, keepaspectratio]{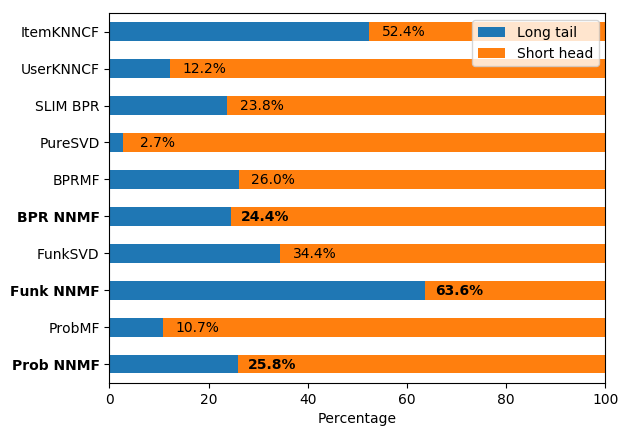}
    \end{subfigure}
\end{figure*}
\begin{figure*}[h]\ContinuedFloat
    \begin{subfigure}[b]{0.32\textwidth}
        \caption{CiteULike}
        \includegraphics[width=0.95\textwidth, keepaspectratio]{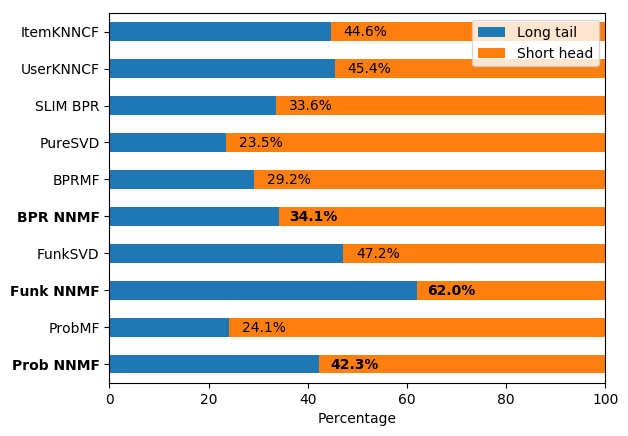}
    \end{subfigure}
    \centering
    \begin{subfigure}[b]{0.32\textwidth}
        \caption{LastFM}
        \includegraphics[width=0.95\textwidth, keepaspectratio]{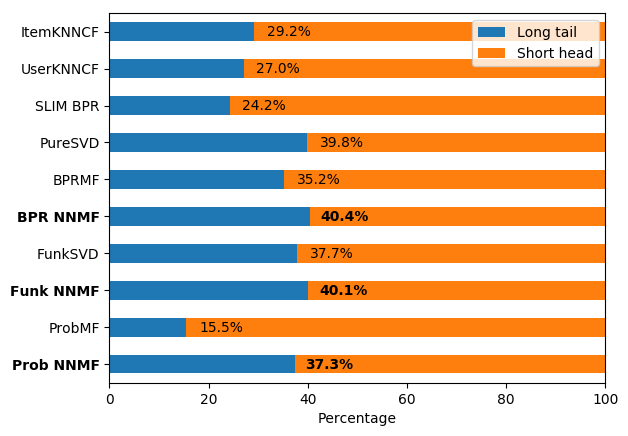}
    \end{subfigure}
    \begin{subfigure}[b]{0.32\textwidth}
        \caption{Movielens 1M}
        \includegraphics[width=0.95\textwidth, keepaspectratio]{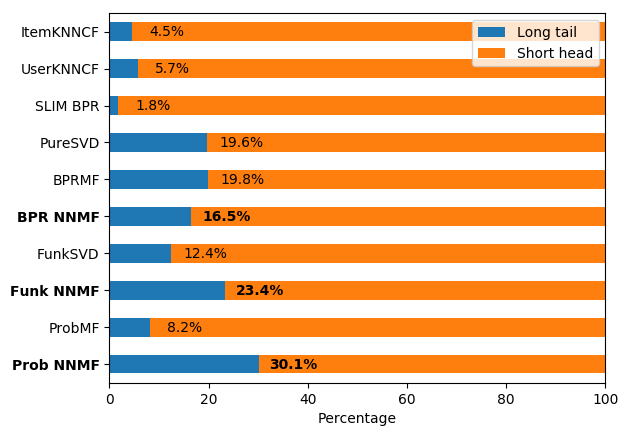}
    \end{subfigure}
\end{figure*}

%\newpage

\section{Top-n performance}
\label{appendix:topn-performance}
We measure the performance on the algorithm on the top-n recommendation task. We carry out the same experiment explained in long-tail accuracy, without removing the head from the test set. %We carry out a significance test with $p-$value=0.01 for NNMFs v MFs comparisons.

% \begin{table*}[h]
%         \centering
%              \caption{Top-n performance. We measure MAP with cutoff at 5. Bold indicates the best performing algorithm. Underline indicates who is best among MF and NNMF, pairwise, in case the difference is statistically significant.}
% \begin{tabular}{c|ccccccc}
% \toprule 
% \textbf{Algorithm} & \textbf{LastFM}&\textbf{Mov1M}&\textbf{BookCr} & \textbf{Pin} &\textbf{Epinions}&\textbf{CiteUL}\\\midrule 
% ItemKNNCF & 0.1235 & \textbf{0.1601} & \textbf{0.0321} & \textbf{0.0328} & \textbf{0.0216} & 0.0873 \\ 
% UserKNNCF & 0.1130 & 0.1591 & 0.0310 & 0.0315 & 0.0209 & 0.0948 \\ 
% SLIM BPR & 0.1246 & 0.1580 & 0.0215 & 0.0323 & 0.0181 & \textbf{0.1004} \\ 
% PureSVD & 0.0726 & 0.1311 & 0.0206 & 0.0265 & 0.0135 & 0.0645 \\ \midrule 
% BPRMF & \textbf{0.1310} & \underline{0.1597} & 0.0159 & 0.0273 & 0.0174 & \underline{0.0745} \\  
% BPR NNMF & 0.1272 & 0.1512 & \underline{0.0215} & \underline{0.0283} & \underline{0.0189} & 0.0691 \\ \midrule 
% FunkSVD & 0.1186 & 0.1058 & 0.0104 & 0.0226 & 0.0082 & 0.0732 \\  
% Funk NNMF & 0.1200 & \underline{0.1367} & \underline{0.0121} & \underline{0.0271} & \underline{0.0175} & 0.0713 \\ \midrule 
% ProbMF & 0.1101 & \underline{0.1564} & 0.0122 & 0.0256 & 0.0090 & \underline{0.0710} \\  
% Prob NNMF & \underline{0.1184} & 0.1425 & \underline{0.0188} & \underline{0.0275} & \underline{0.0171} & 0.0654 \\  
% \bottomrule \end{tabular}
%  \label{table:top_n_5_MAP_0.66_apx}
% \end{table*}

\setlength{\tabcolsep}{2pt}
\begin{table*}[h]
\footnotesize
\centering
\caption{Top-n performance. We measure MAP with cutoff at 5. Bold indicates the best performing algorithm. Underline indicates the best between MF and NNMF, pairwise.}
\begin{tabular}{c|cc|cc|cc|cc|cc|cc|cc|cc|cc|cc}
\toprule 
\multirow{3}{*}{\textbf{Algorithm}} & \multicolumn{4}{c}{\textbf{LastFM}} & \multicolumn{4}{c}{\textbf{Movielens1M}} & \multicolumn{4}{c}{\textbf{BookCrossing}} & \multicolumn{4}{c}{\textbf{Pinterest}} & \multicolumn{4}{c}{\textbf{CiteULike}} \\
 & \multicolumn{2}{c|}{\textbf{MAP}} & \multicolumn{2}{c}{\textbf{Recall}}& \multicolumn{2}{c|}{\textbf{MAP}} & \multicolumn{2}{c}{\textbf{Recall}}& \multicolumn{2}{c|}{\textbf{MAP}} & \multicolumn{2}{c}{\textbf{Recall}}& \multicolumn{2}{c|}{\textbf{MAP}} & \multicolumn{2}{c}{\textbf{Recall}}& \multicolumn{2}{c|}{\textbf{MAP}} & \multicolumn{2}{c}{\textbf{Recall}} \\ 
 & @5 & @20 & @5 & @20& @5 & @20 & @5 & @20& @5 & @20 & @5 & @20& @5 & @20 & @5 & @20& @5 & @20 & @5 & @20 \\ \midrule
 ItemKNNCF & 0.124 & 0.116 & 0.121 & 0.293 & 0.160 & 0.107 & 0.070 & 0.186 & 0.032 & 0.028 & 0.034 & 0.064 & 0.033 & 0.041 & 0.049 & 0.141 & 0.087 & 0.086 & 0.096 & 0.212 \\  
UserKNNCF & 0.113 & 0.107 & 0.112 & 0.273 & 0.159 & 0.115 & 0.076 & 0.215 & 0.031 & 0.028 & 0.036 & 0.071 & 0.032 & 0.039 & 0.047 & 0.136 & 0.095 & 0.096 & 0.105 & 0.228 \\ 
SLIM BPR & 0.125 & 0.117 & 0.123 & 0.291 & 0.158 & 0.108 & 0.074 & 0.199 & 0.021 & 0.020 & 0.026 & 0.052 & 0.032 & 0.040 & 0.049 & 0.139 & 0.100 & 0.101 & 0.115 & 0.236 \\ 
PureSVD & 0.073 & 0.065 & 0.077 & 0.187 & 0.131 & 0.090 & 0.062 & 0.171 & 0.021 & 0.018 & 0.023 & 0.046 & 0.027 & 0.032 & 0.040 & 0.114 & 0.065 & 0.061 & 0.067 & 0.157 \\ \midrule
BPRMF & 0.131 & 0.125 & 0.129 & 0.306 & 0.160 & 0.111 & 0.071 & 0.201 & 0.016 & 0.016 & 0.021 & 0.052 & 0.027 & 0.034 & 0.042 & 0.124 & 0.074 & 0.075 & 0.084 & 0.203 \\  
BPR NNMF & 0.127 & 0.121 & 0.127 & 0.303 & 0.151 & 0.106 & 0.067 & 0.195 & 0.021 & 0.020 & 0.025 & 0.060 &0.028 & 0.035 & 0.043 & 0.130 & 0.069 & 0.069 & 0.079 & 0.193 \\ \midrule 
FunkSVD & 0.119 & 0.114 & 0.118 & 0.293 & 0.106 & 0.071 & 0.049 & 0.142 & 0.010 & 0.010 & 0.013 & 0.031 & 0.023 & 0.030 & 0.037 & 0.119 & 0.073 & 0.078 & 0.093 & 0.208 \\ 
Funk NNMF & 0.120 & 0.116 & 0.122 & 0.294 & 0.137 & 0.094 & 0.063 & 0.184 & 0.012 & 0.013 & 0.018 & 0.045 & 0.027 & 0.035 & 0.042 & 0.130 & 0.071 & 0.079 & 0.089 & 0.218 \\ \midrule 
ProbMF & 0.110 & 0.106 & 0.114 & 0.280 & 0.156 & 0.110 & 0.072 & 0.201 & 0.012 & 0.012 & 0.016 & 0.045 & 0.026 & 0.032 & 0.040 & 0.119 & 0.071 & 0.072 & 0.084 & 0.200 \\ 
Prob NNMF & 0.118 & 0.114 & 0.120 & 0.292 & 0.142 & 0.099 & 0.065 & 0.189 & 0.019 & 0.019 & 0.026 & 0.061 &0.027 & 0.034 & 0.042 & 0.125 & 0.065 & 0.068 & 0.077 & 0.196 \\ 
 \bottomrule
\end{tabular}
 \label{table:top_n_5_MAP_0.66_apx}
\end{table*}
\setlength{\tabcolsep}{5pt}

%\newpage

\section{Performance varying item popularity range}
\label{appendix:stability-per-popularity}
We divide the items in popularity ranges identified by long tail cuts. We compute a value as the avg of the jaccard index the items in every one of those ranges.

\begin{figure*}[h]
    \centering
    \begin{subfigure}[b]{0.32\textwidth}
        \caption{BookCrossing}
        \includegraphics[width=0.95\textwidth, keepaspectratio]{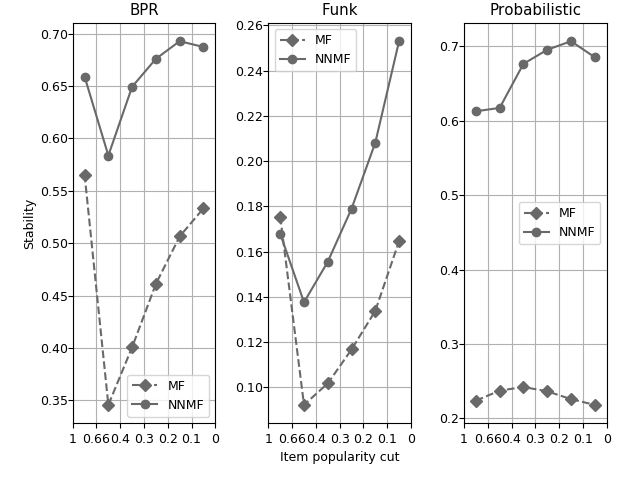}
    \end{subfigure}
    \begin{subfigure}[b]{0.32\textwidth}
        \caption{CiteULike}
        \includegraphics[width=0.95\textwidth, keepaspectratio]{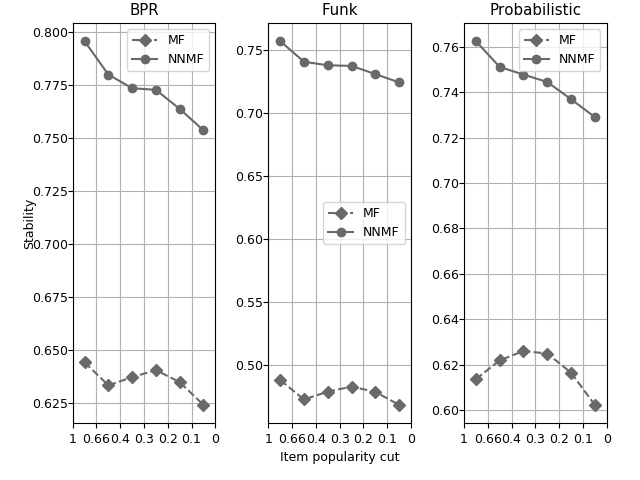}
    \end{subfigure}
    \centering
    \begin{subfigure}[b]{0.32\textwidth}
        \caption{Epinions}
        \includegraphics[width=0.95\textwidth, keepaspectratio]{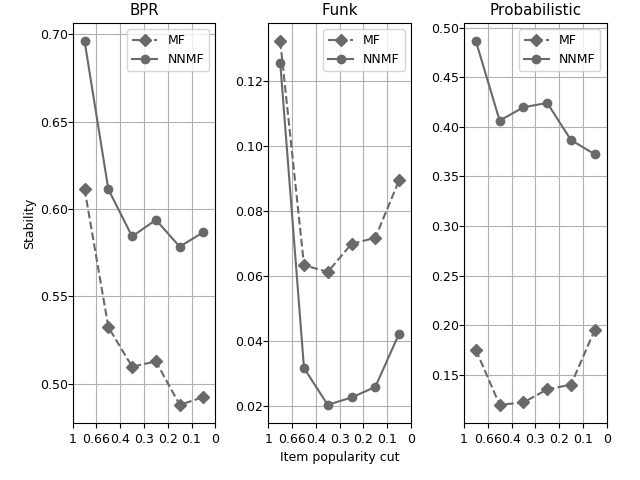}
    \end{subfigure}
\end{figure*}
\begin{figure*}[h]\ContinuedFloat
    \begin{subfigure}[b]{0.32\textwidth}
        \caption{LastFM}
        \includegraphics[width=0.95\textwidth, keepaspectratio]{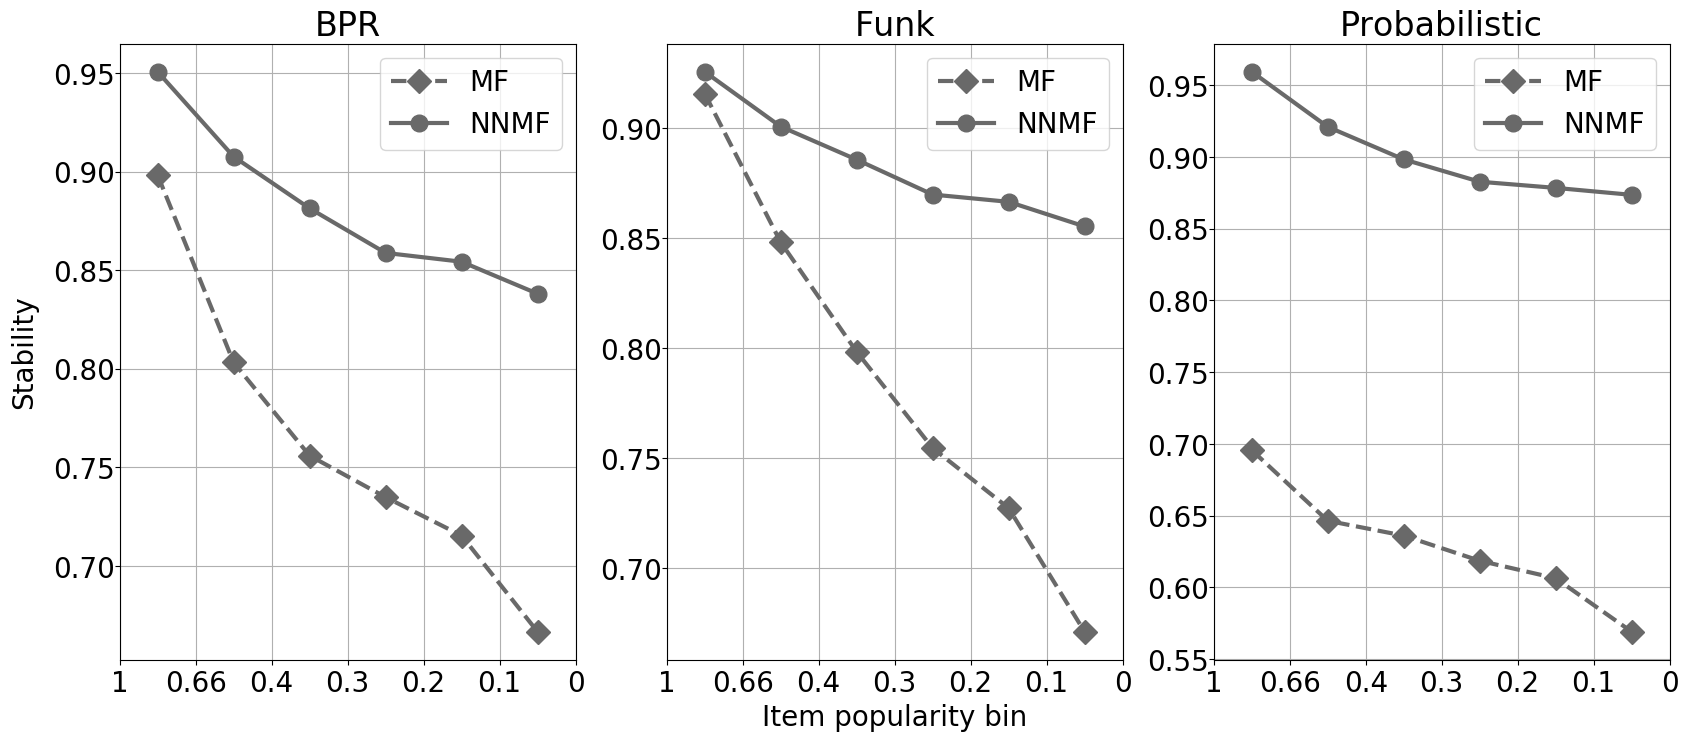}
    \end{subfigure}
    \centering
    \begin{subfigure}[b]{0.32\textwidth}
        \caption{Movielens 1M}
        \includegraphics[width=0.95\textwidth, keepaspectratio]{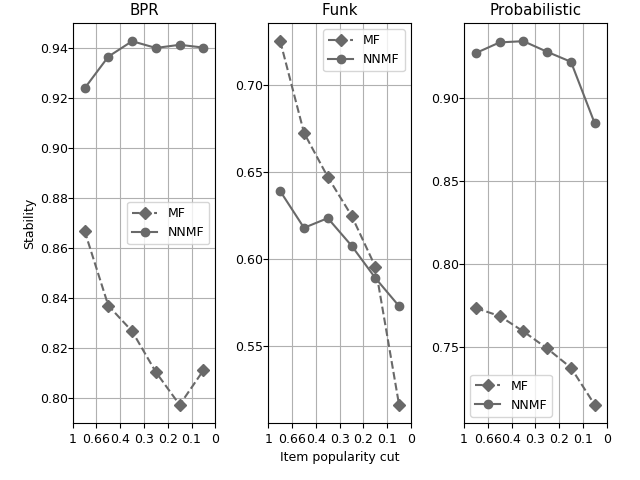}
    \end{subfigure}
    \begin{subfigure}[b]{0.32\textwidth}
        \caption{Pinterest}
        \includegraphics[width=0.95\textwidth, keepaspectratio]{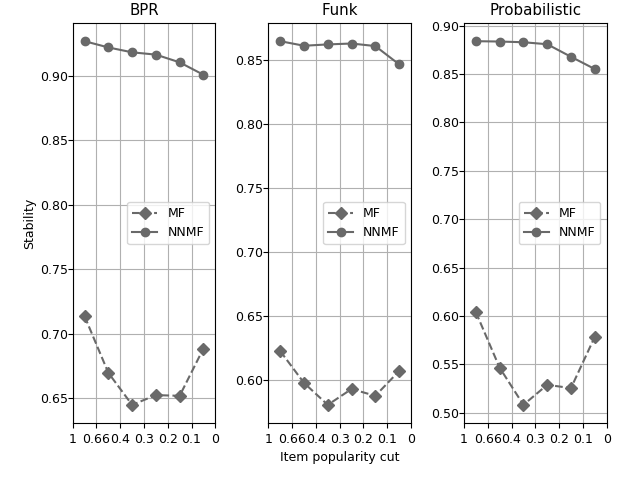}
    \end{subfigure}
\end{figure*}

\section{Training time}
\label{appendix:training-time}

\begin{table*}[h] \centering \caption{Training time in minutes.} \begin{tabular}{c|c|c|c|c|c|c} \toprule \textbf{Algorithm} & \textbf{\lastfm} & \textbf{\movielensom} & \textbf{\bookcrossing} & \textbf{\pinterest} & \textbf{\epinions} & \textbf{\citeulike} \\ \midrule 
\bprmf & 1.4 ± 0.004 & 8.2 ± 0.682 & 8.7 ± 0.893 & 28.2 ± 2.505 & 10.1 ± 1.082 & 4.9 ± 0.600 \\ 
\bprnnmf & 5.1 ± 0.130 & 6.0 ± 0.023 & 29.2 ± 0.179 & 70.2 ± 2.041 & 46.4 ± 0.130 & 2.4 ± 0.019 \\ \midrule 
\funkmf & 0.5 ± 0.002 & 0.4 ± 0.002 & 6.7 ± 0.079 & 20.9 ± 0.039 & 3.9 ± 0.009 & 1.9 ± 0.006 \\ 
\funknnmf & 1.0 ± 0.011 & 100.3 ± 1.311 & 10.2 ± 0.051 & 42.7 ± 0.399 & 22.9 ± 0.065 & 4.7 ± 0.022 \\ \midrule 
\pmf & 1.2 ± 0.002 & 6.4 ± 0.023 & 10.8 ± 0.064 & 26.5 ± 0.078 & 2.8 ± 0.016 & 8.5 ± 0.053 \\ 
\pnnmf & 2.4 ± 0.010 & 6.5 ± 0.157 & 62.5 ± 0.437 & 40.4 ± 0.343 & 54.7 ± 1.151 & 4.4 ± 0.018 \\ \bottomrule 
\end{tabular} \label{table:training_time} \end{table*}
